# Supplementary material for: Bandits Meet Mechanism Design to Combat Clickbait in Online Recommendation
Source: arXiv:2311.15647 source file (2023-11-27)
Supplement: Supplementary file 1 [file appendix.tex]

\input{sections/proofs}

\newpage

\section*{Notes (can be deleted)}

\begin{align*}
    \E_\bd [n_T(\mu, i)] \geq \frac{\log(T)}{\Delta_i^2}
\end{align*}
So, 
\begin{align*}
    \E_\bd [n_T(i)] = \frac{\E_\bd [n_T(\mu, i)]}{d_i} \geq \frac{\log(T)}{d_i \Delta_i^2}
\end{align*}

\section*{Notation} 

\begin{itemize}
    \item "click-through rate, marketing value, arm strategies": \quad $d_1, \dots, d_K$. Maybe, instead: 
    $s_1, \dots, s_K$
    \item "post-click feedback, post-click reward, follow-up reward, true value": \quad $\mu_1, \dots, \mu_K$.
    \item "mixed arm strategies": \quad $\sigma_1, \dots, \sigma_K$ 
    \item "desired strategy given $\mu$": \quad $\s(\mu)$
    \item "welfare function, principal's utility": \quad $u(\s, \mu)$
    \item "arm's private value per-click": \quad $\nu_1, \dots, \nu_K$
    \item "arm $i$'s utility, arm's surplus": \quad $S_i(d_i, \s_{-i})$
    \item Strategic Regret of $M$ and $\bs$: $R_T(M, \bs)$ 
    \item Strong Strategic Regret: $R^S_T (M) = \max_{\bs\in \NE(M)} R_T(M, \bs)$
    \item Weak Strategic Regret: $R^W_T(M) = \min_{\bs \in \NE(M)} R_T(M, \bs)$ 
\end{itemize}

\section{Auxiliary Lemmas}

\begin{lemma}
The welfare function $u(\s, \mu) = \s\mu - \lambda (\s-\mu)^2$ is $5\lambda$-Lipschitz w.r.t.\ the $\ell_1$-norm. 
\end{lemma}
\begin{proof}
\begin{align*}
    | u(d_1, \mu_1) - u(d_2, \mu_2) | & \leq |d_1 \mu_1 - d_2 \mu_2| + \lambda | (d_1 - \mu_1)^2 - (d_2 - \mu_2)^2| \\ 
    & \leq | d_1  - d_2| + | \mu_1 - \mu_2| + \lambda | (d_1 - \mu_1) + (d_2 - \mu_2)| |(d_1 - \mu_1) - (d_2 - \mu_2)| \\ 
    & \leq | d_1  - d_2| + | \mu_1 - \mu_2| + 4 \lambda (| d_1 - d_2| + |\mu_1 - \mu_2| ) \\
    & \leq 5\lambda ( | d_1 - d_2| + | \mu_1 - \mu_2|). 
\end{align*}
\end{proof}

\begin{lemma}
For any Nash equilibrium $(d_1, \dots, d_K)$ under UCB-S, we have
$d_i \geq \s(\mu_i) - O(1/T^2)$. 
\end{lemma}

\begin{proof}
Applying Hoeffding's inequality twice, it follows that with probability $1-1/T^2$ it holds for any $d_i \leq \s(\mu_i)$ that
\begin{align*}
    \underline d_i^t \leq d_i \leq \s(\mu_i) \leq \max_{\mu \in [\underline \mu_i^t, \overline \mu_i^t]} \s(\mu)
\end{align*}
for all $t \in [T]$. Hence, $i \in A_t$ for all $t \in [T]$ with probability $1-1/T^2$ for any $d_i \leq \s(\mu_i)$. Let $\mathcal{E}_i = \{ i \in A_t \, \forall t \in [T]\}$. 
Suppose that $d_i < \s(\mu_i) - \s(\mu_i) / T^2$. For any $\s_{-i}$, we then have 
\begin{align*}
    S_i(\s(\mu_i), \s_{-i}) & = \E \left[ n_T(i) \mid (\s(\mu_i), \s_{-i}) \right] \s(\mu_i) \mu_i \\ 
    & \geq \E \left[ n_T(i) \mid (\s(\mu_i), \s_{-i}), \mathcal{E}_i \right] \s(\mu_i) \mu_i (1- 1/T^2)  \\
    & > \E \left[ n_T(i) \mid (\s(\mu_i), \s_{-i}), \mathcal{E}_i \right] d_i \mu_i \\ 
    & = \E \left[ n_T(i) \mid (d_i, \s_{-i}), \mathcal{E}_i \right] d_i \mu_i \\
    & \geq \E \left[ n_T(i) \mid (d_i, \s_{-i})\right] d_i \mu_i = S_i (d_i, \s_{-i}),
\end{align*}
where in the second last line we used that  $\E \left[ n_T(i) \mid (d_i, \s_{-i}), \mathcal{E}_i \right] = \E \left[ n_T(i) \mid (\s'_i, \s_{-i}), \mathcal{E}_i\right]$ for all choices of $d_i, \s'_i \in [0,1]$ and $\s_{-i}\in [0,1]^{K-1}$ and $\E[n_T(i) \mid \bd, \mathcal{E}_i] \geq \E[n_T(i) \mid \bd]$ for any $\bd \in [0,1]^K$. This means that $\s(\mu_i)$ strictly dominates every $d_i < \s(\mu_i) - 1/T^2$. Hence, any Nash equilibrium $\bd = (d_1, \dots, d_K)$ must satisfy $d_i \geq \s(\mu_i) - 1/T^2$ for all $i \in [K]$. 
\end{proof}

\begin{lemma}[Existence of NE under UCB-S]
Under mechanism UCB-S, there exists a Nash equilibrium for the arms. 
\end{lemma}

\begin{proof}
The strategy set $[0,1]$ is compact and for Glickberg's theorem~\cite{glicksberg1952further} to apply we need to show the continuity of $S_i(\bd)$ under mechanism UCB-S. 
\end{proof}

\begin{lemma}[Existence of NE under Oracle Mechanisms]
Under both oracle mechanisms in Proposition~\ref{prop:oracles} there exists a Nash equilibrium for the arms. 
\end{lemma}

\begin{proof}
For the first oracle mechanism in Proposition~\ref{prop:oracles}, the existence of a Nash equilibrium is obvious (could for example shown via Glickberg's theorem using that $S_i(\bd)$ is continuous under the mechanism). 

Under the second oracle mechanism in Proposition~\ref{prop:oracles}, the surplus function $S_i(\bd)$ is \emph{not} continuous. However, the existence of a NE can be shown directly. Suppose that the second best arm $j^*$ plays $\s_{j^*} = \s(\mu_{j^*})$. Then, for arm $i^*$ the best response is the largest $\s_{i^*}$ such that $u(\s_{i^*}, \mu_{i^*}) > u(\s(\mu_{j^*}), \mu_{j^*})$. We see that any strategy profile $\s_{-i^*} \in [0,1]^{K-1}$ are then a best response to $\s_{i^*}$ (especially, $\s_{j^*} = \s(\mu_{j^*})$ for $j^*$), since they will never be selected by the oracle mechanism given that $i^*$ plays the $\s_{i^*}$ from above. Hence, the pure strategies $(d_1, \dots, d_K)$ with $\s_{i^*}$ from above, $\s_{j^*} = \s(\mu_{j^*})$, and arbitrary remaining strategies form a Nash equilibrium. 

\textcolor{purple}{This is actually not a valid way to describe a NE, because the described strategy $\s_{i^*}$ has to move arbitrary close to $\s_{j^*}$. We can make a statement like: Let $\varepsilon>0$ be arbitrarily small. Suppose that the arms play an $\varepsilon$-NE. etc.}
\end{proof}
